# Supplementary material for: Climate Modelling in Low-Precision: Effects of both Deterministic & Stochastic Rounding
Source: arXiv:2104.15076 source file (2021-04-30)
Supplement: Supplementary file 1 [file supplement.tex]

%%%%%%%%%%%%%%%%%%
%%%BEGIN FIGURE%%%%%%%
%%%%%%%%%%%%%%%%%%
%
%\begin{figure}
%	\centering
%	\includegraphics[width=.5\linewidth]{ElNinoAnomaly.pdf}
%	\captionsetup{width=.9\linewidth}
%	\caption{El Ni\~no SST anomaly.}
%	\label{fig:ElNinoAnomaly}
%\end{figure}
%
%%%%%%%%%%%%%%%%%%
%
%
%\begin{figure}
%\centering
%	\begin{subfigure}{\linewidth}
%		\includegraphics[width=\textwidth]{GPWD_TP_logrelerr_SPPTSR.pdf}
%		\label{fig:TP_LRE}
%	\end{subfigure}
%%
%	\begin{subfigure}{\linewidth}
%		\includegraphics[width=\textwidth]{GPWD_TP_AbsErr.pdf}
%		\label{fig:TP_AE}		
%	\end{subfigure}
%%
%\captionsetup{width=.9\linewidth}
%\caption{Grid-projected Wasserstein distance maps (cf.\ \eqref{eq:LRE} and \eqref{eq:AE} resp.)}
%\end{figure}
%
%%%%%%%%%%%%%%%%%%
%
%\begin{figure}
%\centering
%\includegraphics[width=.8\linewidth]{mongecon_totprecip_1500samples.pdf}
%\caption{Results from sampling the global precipitation distribution.}
%\end{figure}
%
%%%%%%%%%%%%%%%%%%
%%%%END FIGURE%%%%%%%
%%%%%%%%%%%%%%%%%%
